# Supplementary material for: A two-dimensional stabilized discontinuous Galerkin method on curvilinear embedded boundary grids
Source: arXiv:2102.01857 source file (2021-12-06)
Supplement: Supplementary file 1 [file supplementary_materials.pdf]

# A TWO-DIMENSIONAL STABILIZED DISCONTINUOUS GALERKIN METHOD ON CURVILINEAR EMBEDDED BOUNDARY GRIDS

## SUPPLEMENTARY MATERIAL

ANDREW GIULIANI*

In this supplementary material document, we include one-dimensional convergence tests (section S1), proofs of the conservation and $p$-exactness claims (section S2), and algorithmic details used to avoid precomputing set $W_{i,j}$ (section S3). Equations and figures referenced in the main document retain the same numbering here.

**S1. One-dimensional convergence tests.** We present a convergence tests on nonuniform grids, where we stabilize each intermediate solution of a non-SSP RK time stepper using state redistribution. In both tests, we solve the linear advection equation

$$
\begin{aligned}
u_t + u_x &= 0 \quad \text{on } [\text{-}1, 1], \\
u(x, 0) &= \cos(\pi x + \pi/3),
\end{aligned}
\tag{S1}
$$

with periodic boundary conditions on a nonuniform grid using the DG scheme in (3.7) stabilized by state redistribution, where the time step is

$$
\Delta t = \frac{0.9}{2p+1} h \tag{S2}
$$

on all cells, where $h$ is the size of the large cells in the grid. We also provide the errors on a sequence of uniform grids to compare with the solutions stabilized by state redistribution. The Python code that generated these convergence studies is available at https://github.com/andrewgiuliani/PyDGSRD1D. It can be used with other one-dimensional conservation laws and non-uniform grids.

**S1.1. Randomly generated grid.** We use a sequence of random grids inspired by a model problem in [1]. The sequence of grids is generated by concatenating $N-1$ pairs containing one large and one small cell, where the small cell is placed randomly to the left or right of the large cell. In all pairs, the large cell size is $h = 2/N$. The small cell size in the $i$th pair is $\alpha_i h$ where $\alpha_i = (\gamma_i / \sum_k \gamma_k)$, and $\gamma_i$ is randomly sampled from the uniform distribution on $[0, 1]$. With this set up, small cells are allowed to lie adjacent to one another (or be separated by two large cells) and the number of small cells increases with refinement (Figure S1.1c). Due to the choice of volume fraction, $\alpha_i$, the sum of the lengths of the small cells is equal to $h$, $\sum_k \alpha_k h = h$. In total, the nonuniform grid contains $2N-2$ cells on the interval $(-1, 1)$. Merging neighborhoods are associated all cells, where small cells merge with their larger sibling. Finally, we take a time step proportional to the large cells with size $h = 2/N$ given by the formula in (S2). The minimum volume fraction on the sequence of grids used in this convergence test was 2.24e-07.

The $L_1$ and $L_\infty$ errors at the final time $T = 1$ are provided in Figure S1.1, where we observe the expected $p+1$ rate of convergence in both norms. Even though there are many cells that are vastly smaller than the ones used to determine the time step in (S2) and the number of small cells grows with refinement, state redistribution allows us to explicitly time step in a stable manner. The errors on the nonuniform grids are slightly larger, however, since the merging neighborhoods are all approximately $h$ in size, the difference is not significant.

**S1.2. Two small cells.** We use the nonuniform grid in Figure S1.2c), which is similar to the grid in Figure 3.1. This grid has $2N+3$ cells where $2N+1$ cells have size $h$ and the remaining two cells can be arbitrarily small with size $\alpha h$, where $0 < \alpha < 1$ is small. On the grid, cell $K_0$ is centered at $x = 0$

*Courant Institute, New York University, 251 Mercer St., New York, NY 10012 (giuliani@cims.nyu.edu)

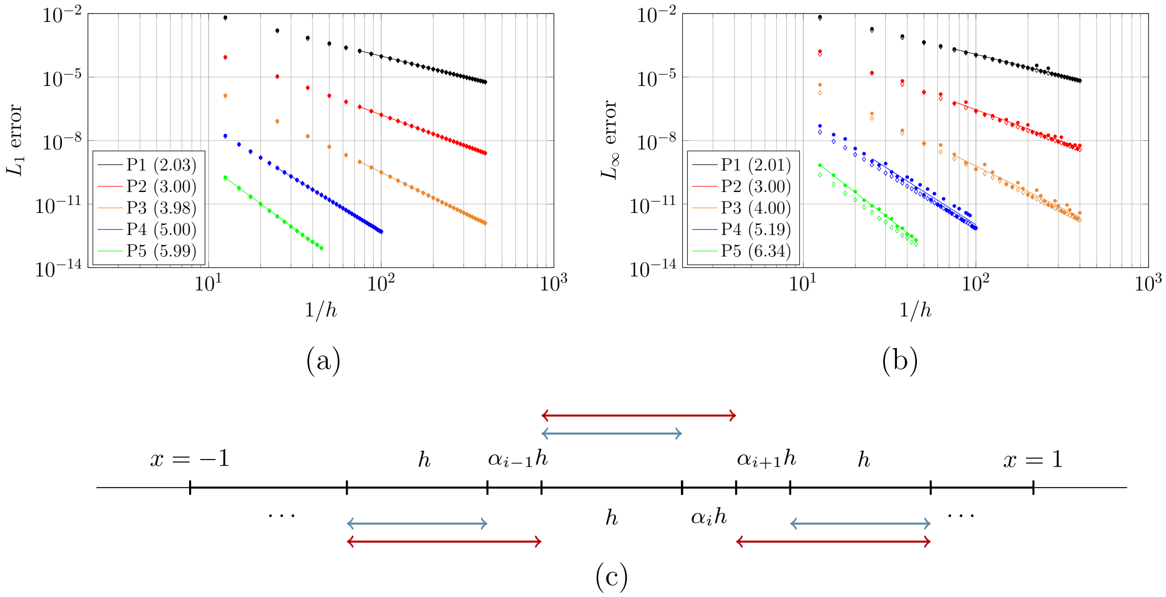


FIG. S1.1. *In a) and b), we provide the $L_1$ and $L_\infty$ errors respectively, at the final time $T = 1$ on both the randomly generated nonuniform grid in c) and the unsplit uniform grid. The errors on the nonuniform grid are plotted with a solid ($\bullet$), and on the uniform grid with a hollow diamond ($\Diamond$). The $L_1$ errors on the nonuniform and uniform grids are visually indistinguishable from one another. The distinction between the two grids is slightly more pronounced in the $L_\infty$ errors. State redistribution does not affect the rate of convergence at the small cells since we observe the expected $p + 1$ rate of convergence in both the $L_1$ and $L_\infty$ norms.*

and $h = 2/(2N + 1 + 2\alpha)$ with $\alpha = 10^{-5}$. Each small cell merges to the left and right and have length $2h + \alpha h$, approximately twice the size of the regular grid cells.

The $L_1$ and $L_\infty$ errors at the final time $T = 1$ on this nonuniform grid and a sequence of uniform grids are provided in Figure S1.2. Even though there are two cells that are vastly smaller than the ones used to determine the time step in (S2), state redistribution allows us to explicitly time step in a stable manner. In S1.2, we observe the expected $p + 1$ rate of convergence in both norms although the error on the nonuniform grid is larger. This difference is only apparent in the $L_1$ norm for high orders of approximation ($p = 4, 5$), though the the errors appear to approach one another with refinement. The difference is more visible in the $L_\infty$ norm for all orders of approximation and does not disappear with refinement. This is not surprising as the merging neighborhoods are more than twice the size of a regular grid cell.

**S2. Accuracy and conservation.** In this section, we show that state redistribution does not modify polynomial solutions to (2.4), or in other words, it is $p$-exact. We also show that state redistribution is conservative. Similar to finite volume schemes [2], this DG scheme stabilized by state redistribution is not monotone.

**Claim 1: *p*-exactness.** $P$-exactness follows from the fact that each step in the state redistribution algorithm preserves polynomials of degree $p$. Consider the case where the provisionally updated DG solution is a polynomial of degree $p$ on the entire domain $\hat{U}_{i,j}(x, y) = f(x, y)$, with $f \in S^p(\Omega)$, $\forall K_{i,j}$. Projecting the provisionally updated numerical solution onto each weighted merging basis using the weighted inner product $\langle \cdot, \cdot \rangle_{\hat{K}_{i,j}}$, we have that the solution on all merging neighborhoods is the original function $\hat{Q}_{i,j}(x, y) = f(x, y)$, since the merging basis $\{\hat{\varphi}_{i,j,k}\}_{k=0\ldots N_p}$ spans $S^p(\hat{K}_{i,j})$, $\forall K_{i,j}$. Projecting the average of overlapping neighborhood solutions back onto the base grid using the inner product

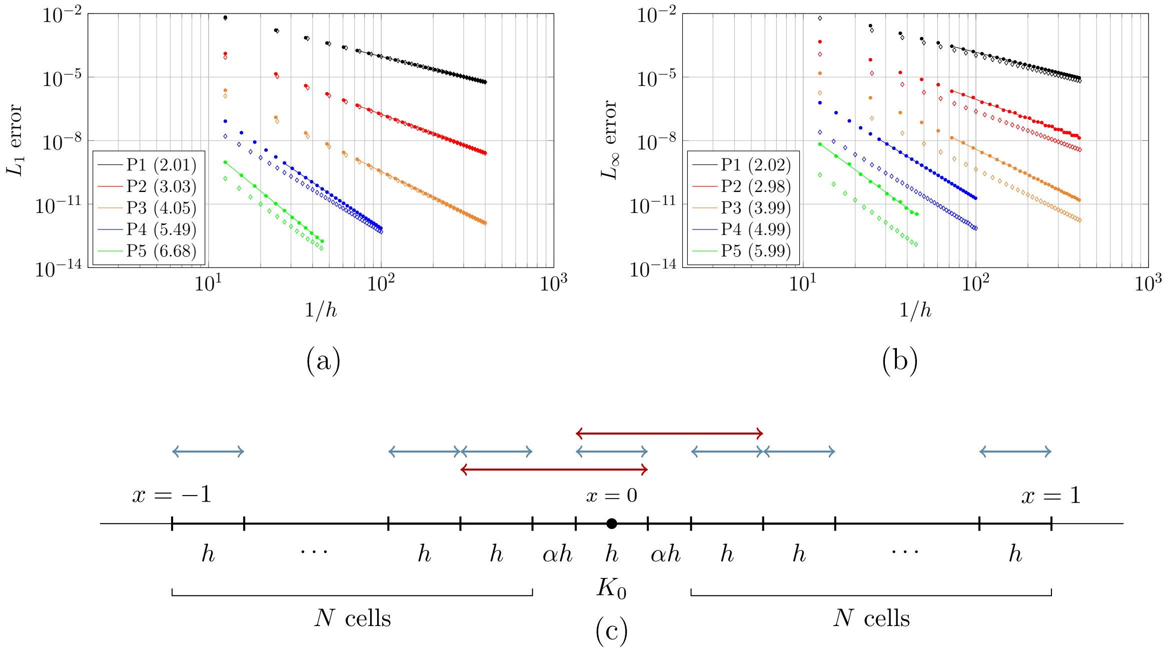


FIG. S1.2. *In a) and b), we provide the $L_1$ and $L_\infty$ errors respectively, at the final time $T = 1$ on the grid shown in c). The errors on the nonuniform grid are plotted with a solid (•), and on the uniform grid with a hollow diamond (◊). State redistribution does not affect the rate of convergence at the small cells since we observe the expected $p+1$ rate of convergence in both the $L_1$ and $L_\infty$ norms. The neighborhoods associated to the large cells are indicated by the blue arrows and those associated to the small cells $K_{-1}$ and $K_1$ are indicated by the red arrows.*

$\langle \cdot, \cdot \rangle_{K_{i,j}}$, the solution in the final update (5.3) remains $U_{i,j}^{n+1}(x, y) = f(x, y)$, since $\text{span}_{k=0\ldots N_p}\{\varphi_{i,j,k}\} = S^p(K_{i,j})$, $\forall K_{i,j}$.

**Claim 2: conservation.** In this section, we adapt the proof presented in [2] to DG methods. The total mass of the DG numerical solution after one forward Euler step of the RK scheme is

$$\text{(S1)} \qquad \begin{aligned} \mathcal{M}^{n+1} &= \sum_{i,j} \int_{K_{i,j}} U_{i,j}^{n+1}(x, y)\, dx\, dy \\ &= \sum_{i,j} |K_{i,j}| c_{i,j,0}^{n+1}, \end{aligned}$$

because $\varphi_{i,j,0} = 1$ and orthogonality of the basis functions. Using the final update (5.3) for the solution coefficient $c_{i,j,0}^{n+1}$ associated to the constant basis function in (S1), we obtain

$$\text{(S2)} \qquad \mathcal{M}^{n+1} = \sum_{i,j} \frac{1}{N_{i,j}} \sum_{(r,s)\in W_{i,j}} \int_{K_{i,j}} \hat{Q}_{r,s}\, dx\, dy.$$

Note that the total mass can also be written as a sum of contributions from each merging neighborhood by rearranging the sum in (S2), i.e.,

$$\text{(S3)} \qquad \mathcal{M}^{n+1} = \sum_{i,j} \hat{\mathcal{M}}_{i,j},$$

where the contribution of merging neighborhood $(i, j)$ is

$$
\begin{aligned}
\hat{\mathcal{M}}_{i,j} &= \sum_{(r,s)\in M_{i,j}} \frac{1}{N_{r,s}} \int_{K_{r,s}} \hat{Q}_{i,j}(x,y)\ dx\ dy, \\
&= |\hat{K}_{i,j}| \langle \hat{Q}_{i,j}, 1\rangle_{\hat{K}_{i,j}}.
\end{aligned} \tag{S4}
$$

Recognizing that the first equation in (S4) is the weighted projection of $\hat{Q}_{i,j}(x,y)$ onto the neighborhood's constant basis function $\hat{\varphi}_{i,j,0} = 1$ scaled by $|\hat{K}_{i,j}|$, we have

$$
\hat{\mathcal{M}}_{i,j} = |\hat{K}_{i,j}| \hat{q}_{i,j,0}, \tag{S5}
$$

Using (5.2) in (S5), we obtain

$$
\hat{\mathcal{M}}_{i,j} = \sum_{(r,s)\in M_{i,j}} \frac{1}{N_{r,s}} \int_{K_{r,s}} \hat{U}_{r,s}\ dx\ dy. \tag{S6}
$$

Substituting the neighborhood contribution (S6) into the expression for total mass on the grid (S3), we have

$$
\mathcal{M}^{n+1} = \sum_{i,j} \sum_{(r,s)\in M_{i,j}} \frac{1}{N_{r,s}} \int_{K_{r,s}} \hat{U}_{r,s}\ dx\ dy. \tag{S7}
$$

This simplifies to

$$
\mathcal{M}^{n+1} = \sum_{i,j} \int_{K_{i,j}} \hat{U}_{i,j}\ dx\ dy, \tag{S8}
$$

and shows that the mass is the same before and after state redistribution.

**S3. Algorithm.** In the main document, it was stated that set $W_{i,j}$ does not in fact need to be precomputed [2] and the action of (5.3) can be implemented using a nested for loop. This is shown in Algorithm S3.1 for DG methods.

**Algorithm S3.1** Implementation of (5.3) without constructing $W_{i,j}$

**for** $i, j, k$ **do**
  $c^{n+1}_{i,j,k} \leftarrow 0$
**end for**
**for** $i, j$ **do**
  **for** $(r, s) \in M_{i,j}$ **do**
    **for** $k = 0 \dots N_p$ **do**
      $c^{n+1}_{r,s,k} \leftarrow c^{n+1}_{r,s,k} + (\int_{K_{r,s}} \varphi_{r,s,k} \hat{Q}_{i,j}\ dx\ dy)/(|K_{r,s}|\ N_{r,s})$
    **end for**
  **end for**
**end for**

REFERENCES

[1] C. Engwer, S. May, A. Nüßing, and F. Streitbürger, "A stabilized DG cut cell method for discretizing the linear transport equation," *SIAM Journal on Scientific Computing*, vol. 42, no. 6, pp. A3677–A3703, 2020.

[2] M. Berger and A. Giuliani, "A state redistribution algorithm for finite volume schemes on cut cell meshes," *Journal of Computational Physics*, vol. 428, p. 109820, 2021.
